# Supplementary material for: Optimizing Airborne Wind Energy with Reinforcement Learning
Source: arXiv:2203.14271 source file (2022-03-27)
Supplement: Supplementary file 1 [file Supplementary_Information.pdf]

# Supplementary information: Optimizing Airborne Wind Energy with Reinforcement Learning

N. Orzan, C. Leone, A. Mazzolini, J. Oyero, A. Celani

## I. DETAILS OF THE SIMULATED ENVIRONMENT: KITE-VEHICLE DYNAMICS

In this section we provide all the calculations regarding the integration of the equations of motion of the kite-vehicle system.

Starting from the equations of motion and the relative constraints as follows:

$$\begin{cases} m\ddot{\mathbf{x}}_k = \mathbf{F}^{aer} + m\mathbf{g} - \mathbf{T} \\ M\ddot{\mathbf{x}}_v = \mathbf{F}^\mu + \mathbf{N} + M\mathbf{g} + \mathbf{T} \\ z_v = 0 \\ |\mathbf{r}(t)| = R \quad \text{where } \mathbf{r} = \mathbf{x}_k - \mathbf{x}_v \end{cases} \quad (1.1)$$

where we explicit the fixed tether length and the position of the vehicle on the ground.

From the equilibrium of the forces on the  $z$  axis for the vehicle, the modulus of the normal reaction of the ground on the vehicle can be written as:

$$N = Mg - T_z.$$

The friction force is exerted between the vehicle and the ground, and is proportional to the sum of the forces acting on the vehicle on the vertical direction:

$$\begin{aligned} |\mathbf{F}^\mu| &= \mu N \\ &= \mu(Mg - T_z) \end{aligned}$$

where  $\mu$  is the friction coefficient.

To solve the system, let us compute the ratio of the first two equations of system 1.1 by the respective masses and subtract the resulting equations:

$$\ddot{\mathbf{r}} = \frac{\mathbf{F}^{aer} - \mathbf{T}}{m} - \frac{\mathbf{F}^\mu + \mathbf{N} + \mathbf{T}}{M}, \quad (1.2)$$

Let's now compute the derivative of  $|\mathbf{r}(t)|$  with respect to time (the time dependence in the following passages is suppressed for clarity):

$$\frac{1}{2} \frac{d}{dt} |\mathbf{r}|^2 = |\mathbf{r}| \mathbf{e}_r \cdot \dot{\mathbf{r}} = \mathbf{r} \cdot \dot{\mathbf{r}} = 0,$$

where  $\mathbf{e}_r$  is the unit vector directed along the cable, labeled by  $\mathbf{r}$ . Deriving a second time we end up with:

$$\ddot{\mathbf{r}} \cdot \mathbf{r} = -\dot{\mathbf{r}}^2$$

We can now equate  $-\dot{\mathbf{r}}^2$  to the product of equation 1.2 with  $\mathbf{r}$ , inserting the constraint of fixed length of the tether indirectly in the system:

$$|\mathbf{T}|R(m^{-1} + M^{-1}) - \frac{\mathbf{F}^{aer} \cdot \mathbf{r}}{m} + \frac{(\mathbf{F}^\mu + \mathbf{N})}{M} \cdot \mathbf{r} = \dot{\mathbf{r}}^2,$$

This equation can be used to find out the modulus of tension force along the rope direction, by writing explicitly both  $\mathbf{N}$  and  $\mathbf{F}^\mu$  as functions of  $|\mathbf{T}|$ :

$$|\mathbf{T}|R(m^{-1} + M^{-1}) = \frac{\mathbf{F}^{aer} \cdot \mathbf{r}}{m} - \frac{(\mathbf{F}^\mu + \mathbf{N})}{M} \cdot \mathbf{r} + \dot{\mathbf{r}}^2$$

The form of the friction force depends on the status of motion of the vehicle. There are three possible situations:

- The vehicle is moving. Then the friction force opposes the speed of the vehicle:

$$\mathbf{F}^\mu = -\mu N \frac{\mathbf{v}_v}{|\mathbf{v}_v|} = -\mu \frac{N}{|\mathbf{v}_v|} (v_{v,x} \hat{\mathbf{x}} + v_{v,y} \hat{\mathbf{y}}).$$

The equation for the tension then becomes:

$$T = \frac{\frac{\mathbf{F}^{aer} \cdot \mathbf{r}}{m} + \dot{\mathbf{r}}^2 - g \left[ z_k - \frac{\mu}{|\mathbf{v}_v|} (v_{v,x} r_x + v_{v,y} r_y) \right]}{R \frac{m+M}{mM} - \frac{\cos(\theta)}{M} \left[ z_k - \frac{\mu}{|\mathbf{v}_v|} (v_{v,x} r_x + v_{v,y} r_y) \right]}.$$

- The vehicle is still and  $|\mathbf{T}_{xy}| \geq |\mathbf{F}_{Max}^\mu|$ . Then the friction force opposes the tether tension on the  $xy$  plane:

$$\mathbf{F}^\mu = -\mu N \frac{\mathbf{T}_{xy}}{|\mathbf{T}_{xy}|} = -\mu \frac{N}{|\mathbf{T}_{xy}|} (T_x \hat{\mathbf{x}} + T_y \hat{\mathbf{y}})$$

yielding

$$T = \frac{\frac{\mathbf{F}^{aer} \cdot \mathbf{r}}{m} + \dot{\mathbf{r}}^2 - g \left[ z_k - \mu(\cos(\phi) r_x + \sin(\phi) r_y) \right]}{R \frac{m+M}{mM} - \frac{\cos(\theta)}{M} \left[ z_k - \mu(\cos(\phi) r_x + \sin(\phi) r_y) \right]},$$

- The vehicle is still and  $|\mathbf{T}_{xy}| < |\mathbf{F}_{Max}^\mu|$ . Then the friction force is equal and opposite to the tether tension on the  $xy$  plane

$$\mathbf{F}^\mu = -\mathbf{T}_{xy}$$

The modulus of the tension in this case becomes:

$$T = \frac{\frac{\mathbf{F}^{aer} \cdot \mathbf{r}}{m} + \dot{\mathbf{r}}^2 - g z_k}{R \frac{m+M}{mM} - \frac{\sin(\theta)}{M} (\cos(\phi) r_x + \sin(\phi) r_y) - \frac{\cos(\theta)}{M} z_k}$$

Expressing the components for the accelerations of kite and vehicle in the three dimensions, one can write:

$$\begin{cases} m\ddot{x}_k = F_x^{aer} - T_x \\ m\ddot{y}_k = F_y^{aer} - T_y \\ m\ddot{z}_k = F_z^{aer} - T_z - mg \\ M\ddot{x}_v = F_x^\mu + T_x \\ M\ddot{y}_v = F_y^\mu + T_y \\ M\ddot{z}_v = 0. \end{cases} \quad (1.3)$$

These equations are integrated using Euler method with integration step  $\Delta t = 0.001$  s. Since the constraint  $|\mathbf{r}(t)| = R$  is inserted indirectly in the dynamics, the distance between vehicle and kite varies after the integration. To avoid this, the kite position is adjusted according to:

$$\mathbf{x}'_k = \mathbf{x}_k + \frac{\mathbf{x}_k - \mathbf{x}_v}{|\mathbf{x}_k - \mathbf{x}_v|} R.$$

## II. DETAILS OF THE SIMULATED ENVIRONMENT: TURBULENT WIND FLOW

The turbulent Couette Channel flow is a shear-driven motion of an incompressible fluid bounded by two parallel walls in relative motion. The governing equations of the velocity field are the incompressible Navier-Stokes equations, that in dimensional form read

$$\begin{cases} \partial_t \mathbf{u} + \mathbf{u} \cdot \nabla \mathbf{u} = -\frac{1}{\rho} \nabla p + \nu \nabla \cdot (\nabla \mathbf{u}) \\ \nabla \cdot \mathbf{u} = 0, \end{cases} \quad (2.1)$$

where  $\rho$  is the fluid density and  $\nu$  is the kinematic viscosity.

In order to deal with dimensionless equations we introduce the following variables:  $\mathbf{x}^* = \frac{\mathbf{x}}{L}$ ,  $\mathbf{u}^* = \frac{\mathbf{u}}{U}$ ,  $t^* = \frac{t}{L/U}$ ,  $p^* = \frac{p}{\rho U^2}$ , where  $U$  and  $L$  are the characteristic velocity and length of the problem in study. In our case we take the height  $2\delta$  of the channel to be the characteristic length and the upper wall velocity  $U_W$  as the characteristic speed. The resulting dimensionless equations are

$$\begin{cases} \frac{\partial \mathbf{u}^*}{\partial t^*} + \mathbf{u}^* \cdot \nabla \mathbf{u}^* = -\nabla p^* + \frac{1}{Re} \nabla \cdot (\nabla \mathbf{u}^*) \\ \nabla \cdot \mathbf{u}^* = 0 \end{cases} \quad (2.2)$$

where the Reynolds number  $Re = \frac{2U_W\delta}{\nu}$  remains the only defining parameter of the flow, determining the ratio between the weight of the inertial force term and the one of the viscous term. As the magnitude of the inertial term continues to increase and eventually becomes much larger than the viscous term, there results a "runaway" flow instability whereby the damping effect is marginalized. Therefore, 3D instabilities form and become rampant as  $Re$  continues to increase. From this critical point on ( $Re > 1500$ ), the flow starts to show the trademarks of turbulence.

The simulation is initially run in a small box with dimensions  $2\pi \times \pi \times 2$  m<sup>3</sup>, respectively corresponding to the length of the  $x, y$  and  $z$  axes. It follows that the characteristic length for this system  $\delta = 1$  m. The upper wall velocity in this configuration is  $U_W = 3$  m/s and the kinematic viscosity  $\nu = 1/10935$  m<sup>2</sup>/s. This results in a Reynolds number  $Re = 65610$ , giving rise to a highly turbulent flow.

Dimensions and wall velocity are later re-scaled in post-processing, resulting in the  $32\pi \times 32\pi \times 100$  m<sup>3</sup> channel that we use for running the learning simulation, together with  $U_W = 30$  m/s.

In fig. 1 and 2 we report the analysis we performed on the final flux, both along time and on a single frame of the flow. Results are in line with those predicted in ref. (3).

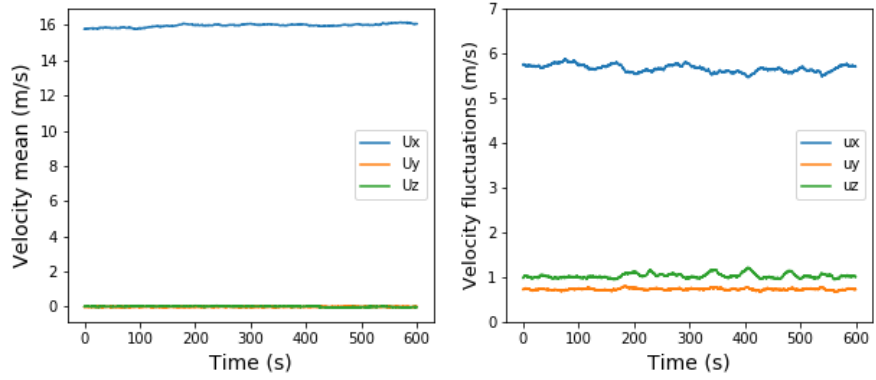

Figure 1. Behaviour of the overall mean and standard deviation of the three components of the velocity plotted with respect to time in seconds from 0 to the entire duration of the flow, being 600s. The mean and the standard deviation are computed by averaging over all the points of the grid at each time step. Each snapshot of the flow is taken at a 0.2s distance from the previous one, resulting in 3000 total frames.

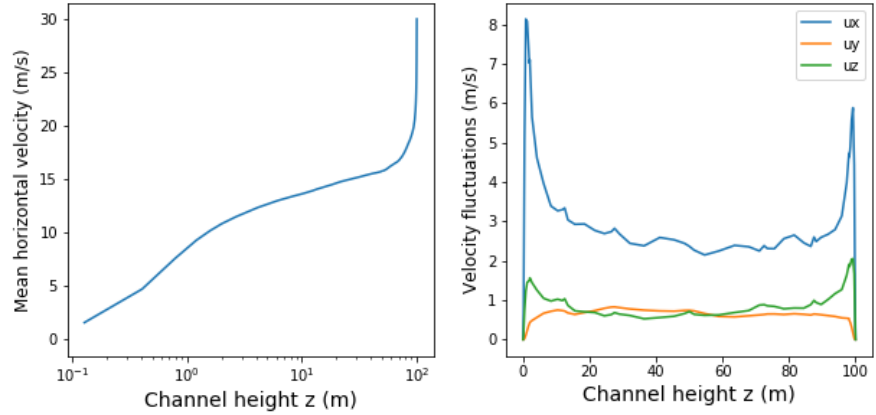

Figure 2. Mean and fluctuations at  $t = 300s$  obtained by averaging over all the grid points of each plane at a fixed channel height  $z$ . As expected the mean velocity scales linearly with height in the viscous sub-layer and then logarithmically afterwards. We portrait just half the channel height in the left plot and the entire spectrum in the right one, in order to highlight the regularity in the mean fluctuations close to the lower and upper walls.

### III. SIMULATION PARAMETERS

Speaking about the values of the parameters employed to simulate the behaviour and the learning of the kite-vehicle system, we first have to disclaim between the *environmental* parameters, such as the physical characteristics of the kite, the duration of the episodes and the magnitude of the penalty, and the *learning* parameters, regarding the magnitude and the scheduling of learning and exploration rate, and the length of the training.

The former ones are resumed in table I and are kept constant in all simulations.

Particular attention must be kept on the control angles  $\alpha$  and  $\psi$  and the perceived angle  $\beta$ . For every simulation we used the discretized attack angles listed in table II with the relative lift and drag coefficients. As for the bank angles we employed  $\psi \in [-15^\circ, 15^\circ]$  and the spacing between adjacent banks is  $\Delta\psi = 3^\circ$ . In the turbulent simulation we account for the angle  $\beta$  between the relative velocity and the  $xy$ -plane as well.

| Parameter                 | Symbol                | Value            |
|---------------------------|-----------------------|------------------|
| Vehicle mass              | $M$                   | $40\text{ kg}$   |
| Kite mass                 | $m$                   | $1\text{ kg}$    |
| Cable length              | $R$                   | $50\text{ m}$    |
| Friction coefficient      | $\mu$                 | $0.4$            |
| Kite area                 | $A$                   | $5\text{ m}^2$   |
| Integration time          | $\Delta t$            | $0.001\text{ s}$ |
| Penalty value             | $P$                   | $1000$           |
| Threshold time for $P$    | $T_{pen}$             | $200\text{ s}$   |
| Penalty threshold for $z$ | $z_{low}$             | $10\text{ m}$    |
| Training ep. duration     | $T$                   | $350\text{ s}$   |
| Evaluation ep. duration   | $T_{eval}$            | $600\text{ s}$   |
| Decision time             | $\Delta t_{decision}$ | $0.25\text{ s}$  |

Table I. Values of the employed environmental parameters for the kite-vehicle system.

The latter is binned uniformly between with  $\beta \in [-80^\circ, 80^\circ]$  with  $\Delta\beta = 20^\circ$ . This amounts to  $8 \times 11 \times 9$  total observables (which represent the states of the learning process) in a turbulent flow, while it is limited to  $8 \times 11$  for simpler flows as we will see later.

| Attack angle $\alpha$ | $C_L(\alpha)$ | $C_D(\alpha)$ |
|-----------------------|---------------|---------------|
| 6                     | 0.65          | 0.05          |
| 8                     | 0.75          | 0.07          |
| 10                    | 0.82          | 0.09          |
| 12                    | 0.9           | 0.1           |
| 14                    | 1.0           | 0.13          |
| 16                    | 1.08          | 0.18          |
| 18                    | 1.1           | 0.18          |
| 20                    | 1.05          | 0.21          |

Table II. Lift coefficient  $C_L$  and drag coefficient  $C_D$  as functions of the attack angle  $\alpha$ . The employed values listed in the table are taken from ref. (3) in the article.

We now shed light on the values of the learning parameters we used for training. Values and scheduling of learning rate and exploration rate are reported in table III and are valid both for trainings through the turbulent channel and for simpler settings. What can be changed is the total number of learning steps  $N_{steps}$ , which is higher for the turbulent trainings as the space of observables is larger and the learning is more difficult.

The scheduling used for the learning rate is

$$\eta_j(S_t, A_t) = \frac{\eta_0}{1 + \left( \frac{n_j(S_t, A_t)}{N_0} \right)^\gamma}$$

and is function of the number of visits  $n_j(S_t, A_t)$  to each observation-action couple. The exploration rate is instead function only of the training time  $j$  and has an initial constant interval  $N_{burn}$  and then shows a power-law decay as follows

$$\epsilon_j = \frac{\epsilon_0 \epsilon_c}{\epsilon_c + (j - N_{burn})^\delta}.$$

A graphic representation of these two power law decays can be found in fig. 3 with  $N_{steps} = 6 \cdot 10^8$ .

As far as the penalty for crashing is concerned, it does not remain the same along one episode: crashing is penalized only during the first 200 s of each episode, with  $P = 1000$  and then is not penalized anymore. The penalty for flying low instead remains the same along the whole episode (and we select  $z_{low} = 10\text{ m}$  as reported in table I). This hard scheduling enhances the finding of a reliable policy to overcome the transient from the initial conditions to the stable pattern.

All the values of the parameters of the simulation with turbulent wind are reported in table III. Time values are expressed in terms of number of learning steps. One learning step follows the other by 0.25 s.

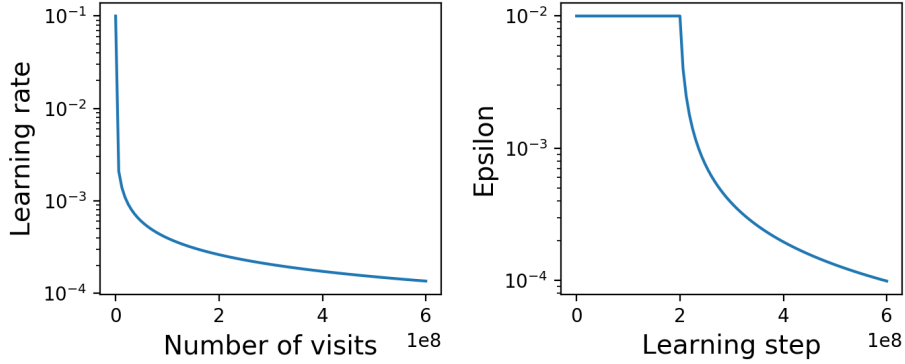

Figure 3. Graphical representation of the scheduling of  $\eta(S_t, A_t)$  and  $\epsilon_t$ . On the left the abscissa represents the number of visits to a certain observation-action couple  $n(S_t, A_t)$  while on the right it is shown the dependence between the exploration rate and the learning step. In this simulation we resort to  $6 \cdot 10^8$  learning steps.

| Parameter    | Value           |
|--------------|-----------------|
| $\eta_0$     | 0.1             |
| $N_0$        | 10000           |
| $\gamma$     | 0.6             |
| $\epsilon_0$ | 0.01            |
| $\epsilon_c$ | $N_{steps}/150$ |
| $N_{burn}$   | $N_{steps}/3$   |
| $\delta$     | 1               |

Table III. Values of the training parameters for any training.  $N_{steps}$  refers to the total number of learning steps of the training and is equal to  $6 \cdot 10^8$  for the turbulent simulations, while  $N_{steps} = 10^7$  for simpler set-ups.

#### IV. LEARNING IN SIMPLER SET-UPS AND WITH DIFFERENT REWARD DISTRIBUTION

As anticipated in section III, we performed various simulations in a simpler environment as well, both as a test bench for the more complex turbulent problem and also in order to try out different reward structures. In this scheme we consider wind velocity to be constant along the  $x$ -axis and uniform. This results in a shorter search for the best strategy, as a much smaller  $N_{steps}$  is needed with respect to the one employed for the trainings in a turbulent environment.

We find out that the system is able to learn effectively (fig. 4) only knowing the value of the control angles. Therefore we can discard the information regarding the angle  $\beta$ , whose knowledge does not improve the performance of the algorithm. This allows us to work with an even more restricted observation-space.

The maximum witnessed return is comparable with the one we witness in the turbulent flow but the parallel is not particularly meaningful either: we selected a constant wind velocity similar to the average velocity measured in the turbulent flow over all the channel, but it is also true that the fraction of the field witnessed by the kite has usually smaller velocity values.

The resulting trajectory is a stable helix-like motion along the episode as portrayed in fig. 7. Also in this case the strategy is stable enough to make the kite remain airborne also for longer periods of time with respect to the ones it has been trained on. As for the turbulent case, we train the kite on episodes of length  $T = 350s$  and then test the policy on longer episodes with  $T_{eval} = 600s$  (cf. table I for all the time intervals employed in the simulations).

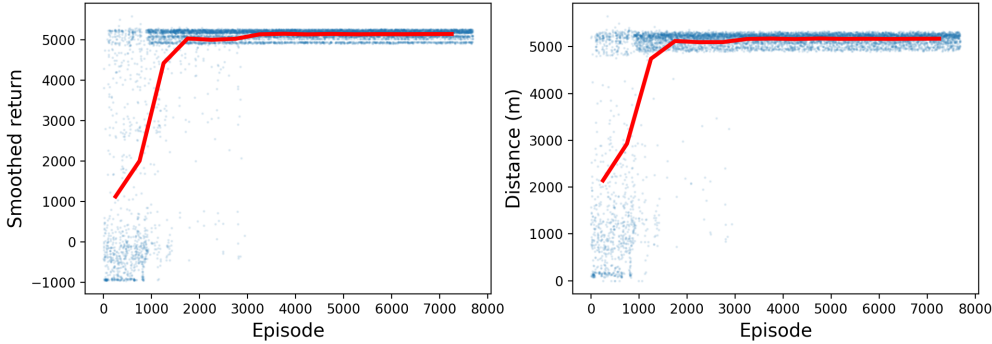

Figure 4. Curve of the return (left) for a training with  $N_{steps} = 10^7$  with constant wind velocity equal to  $15m/s$  along  $x$ , episodes of length  $T = 350s$  and corresponding traveled distances (right), which differ from the return values by the falling penalty and by smaller rewards for  $z_k < z_{low} = 10m$ .

The first test that we perform is the analysis of the best strategy learned at the end of the training. The policy is now easily representable and is reported on the left part fig. 5, where each entry stands for an observation  $S$  and the corresponding arrow is the performed action. Even if this scheme is pretty noisy, we can recognize two stable points with  $\alpha = 8^\circ$  and  $\psi = \pm 12^\circ$  respectively, which act as attractors of the observation-action dynamics. This is made more evident by the right part of fig. 5: if we evaluate the learned strategy, we notice immediately that the two stable points are visited exponentially more times than all the others, resulting in absorbing points of the dynamics.

We can then resort to gather this information and build a simplified policy which drives the dynamics directly towards these two absorbing points avoiding the more intricate cycles portrayed by fig. 5 (left). The new policy that we design is represented in fig. 6.

If we proceed by testing this new policy we find out that the performance is the same as the one obtained at the end of the training, suggesting that the relevant information stands in locating the absorbing points and all the actions that do not point directly there are just the result of noisy learning.

This conclusion is almost analogous to the one drawn in the article with respect to the turbulent flow learning, where the performance of the distilled policy and of the learned one are comparable, nonetheless in that case the transient is responsible for a higher variance.

The other test that we ran in this simple environment is the study of the learning in contexts where the reward structure is different from the original one. If in the main work we award the vehicle for moving as far as possible in the  $x$  direction, here we tried to enquire whether it is possible to make the system move also in other directions even if the wind continues to remain directed along  $x$ .

The obtained results are summarized in fig. 8 and show sensibly smaller returns with respect to the one of fig. 4. This happens since the vehicle is not able to learn efficiently how to exploit the horizontal wind in order to move upwind: it comes out that the followed strategy remains very similar to the original one, with one stable attractor around  $\alpha = 8^\circ$  and  $\psi = 12^\circ$  (fig. 9). The negative absorbing state vanishes since we privilege moving in the positive direction of the  $y$ -axis.

This suggests that the dynamics is not rich enough in order to allow the due plasticity required to the

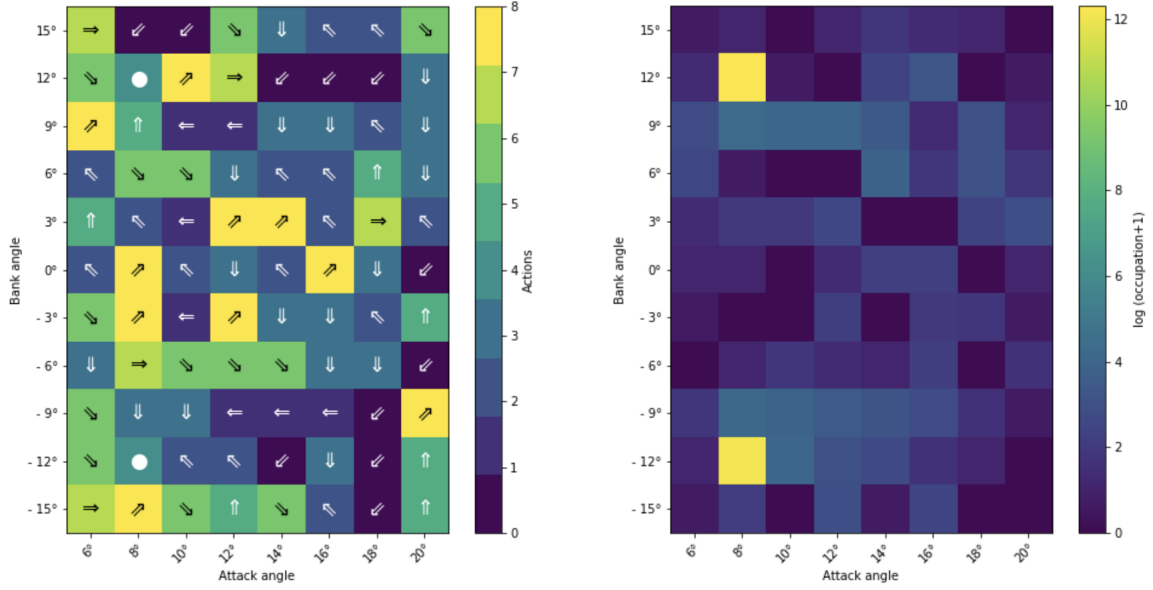

Figure 5. A picture of the best policy learned at the end of the training (left) and the corresponding observation occupation after 166 evaluation episodes (right). Arrows and circles represent the best action to be taken according to the maximization of the learned  $Q$ . The circle stands for keeping attack and bank angles fixed. This figure highlights the presence of two grid-points being the attractors of the observation-action dynamics.

policy in order to make the system move efficiently in a direction which does not correspond to the one given by the wind.

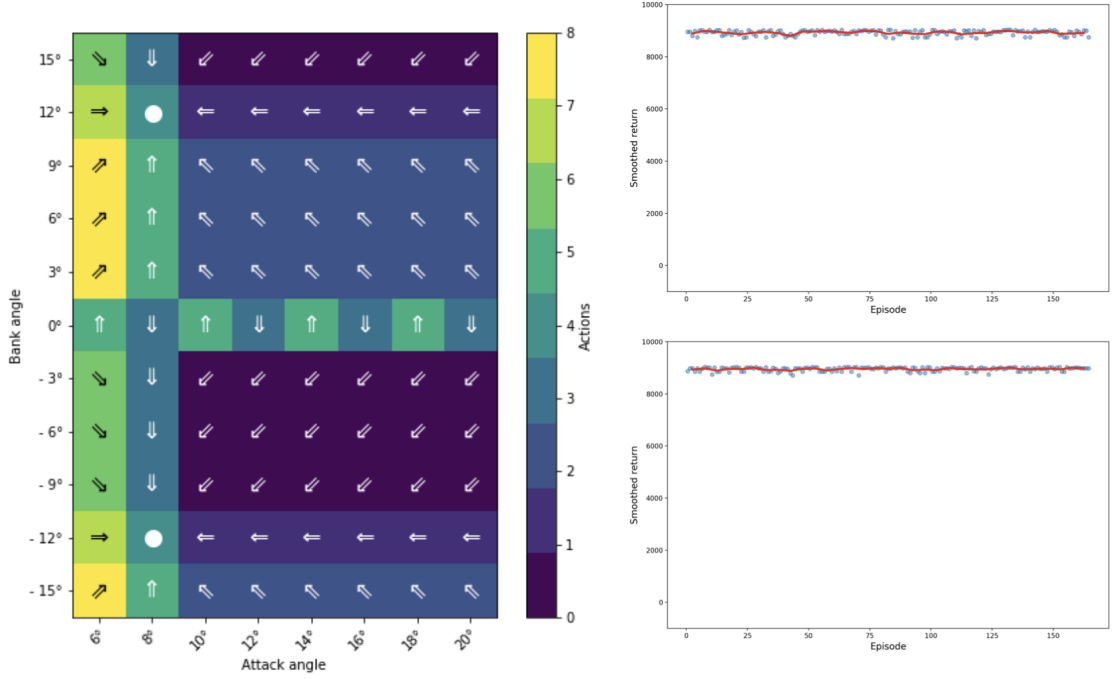

Figure 6. On the left we have the resulting schematized policy obtained by combining the information coming from fig. 5. We drew the shorted path towards the attractors and the performance of the policy is invariate: on the right there are the two plots of the returns collected during the evaluation of the learned policy and of the distilled one for episodes of length  $T = 600$  s.

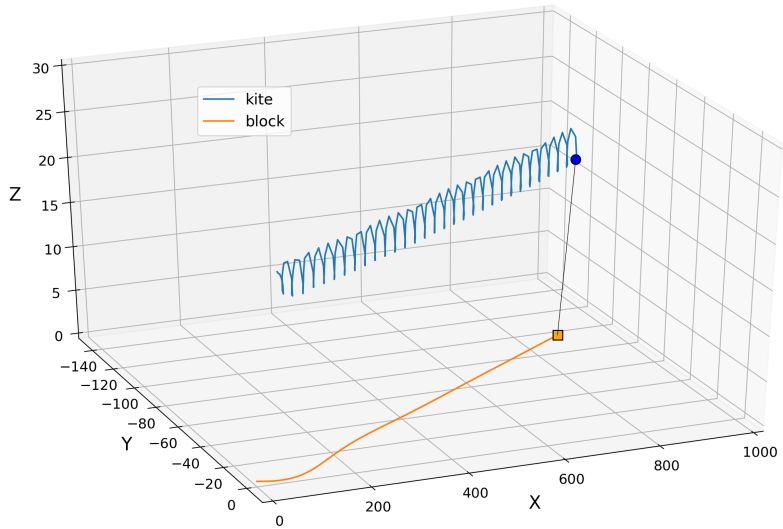

Figure 7. An example of the initial trajectory of the kite-vehicle system evaluated using the learned policy. The helix motion is much more regular than in the turbulent case as the environment is completely predictable and fluctuations are absent.

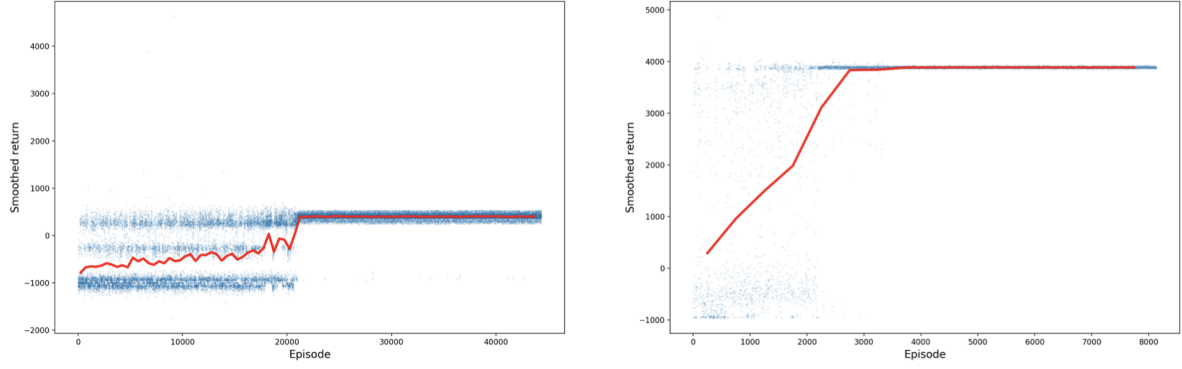

Figure 8. Return growth in a constant wind environment along the  $x$ -axis with a reward that awards the space travelled along  $y$  (left) and the space along the bisectrix of the  $xy$ -plane (right). In both cases the obtained return is sensibly smaller than in the usual reward scheme.

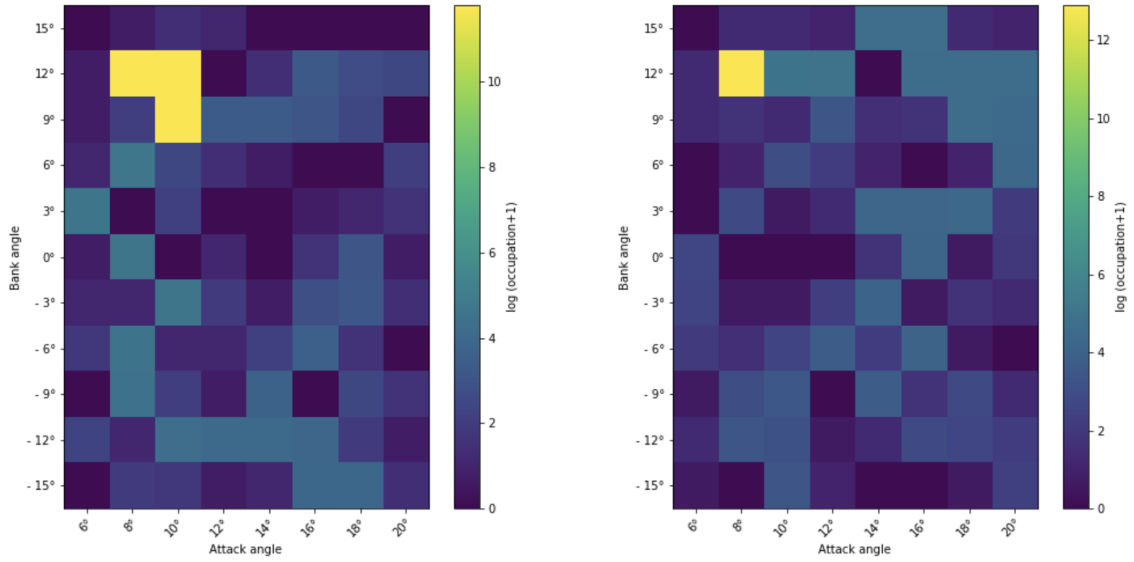

Figure 9. Learning state occupation after evaluation for the case with the reward given along the  $y$ -axis (left) and the reward assigned for the space traveled along the bisectrix of the  $xy$ -plane (right).

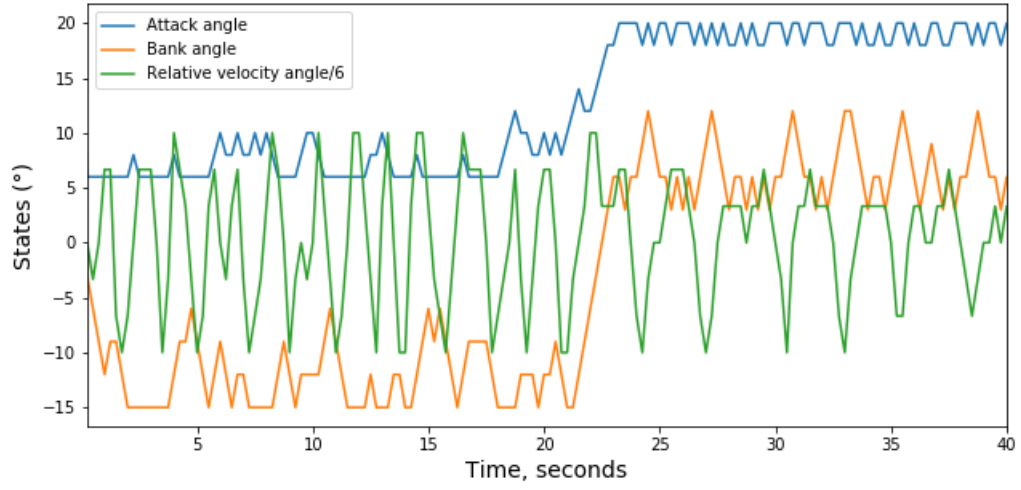

Figure 10. Another example of learning state-action trajectory portraying the beginning of an evaluation episode: in this case the transient phase is much longer and lasts around 20 s before moving to the stationary one.
